# Supplementary material for: On How Zero-Knowledge Proof Blockchain Mixers Improve, and Worsen User Privacy
Source: arXiv:2201.09035 source file (2023-03-06)
Supplement: Supplementary file 1 [file appendix.tex]

\section{Appendices}
% \section{Tracing Adversary Users Case Studies}
\label{sec:tracing-hackers}

In the following, we provide two examples in which we apply our linking results in TC to trace malicious addresses.

\pparagraph{Example 1: Upbit Hackers} On the 27th November 2019, hackers stolen $342{,}000$~\ETH from Upbit, a South-Korean cryptocurrency exchange. As shown in Figure~\ref{fig:trace_upbit_hacker}, \emph{(1)} A depositor \href{https://etherscan.io/address/0xeFf67710a1aE67885f660a965B0A8697CDB161A9}{\texttt{0xeFf...1A9}} receives $1{,}526.95$~\ETH from address \href{https://etherscan.io/address/0x5a88a3aD66234861621e983A498948Ffe6641857}{\texttt{0x5a8...857}}, which obtains the same amount of~\ETH from four labeled Upbit Hacker addresses. \emph{(2)} \href{https://etherscan.io/address/0xeFf67710a1aE67885f660a965B0A8697CDB161A9}{\texttt{0xeFf...1A9}} then deposits $1{,}524$~\ETH into TC~1,~10, and~100~\ETH pools during block $11{,}971{,}221$ and $11{,}972{,}040$. \emph{(3)} From our linking results, we find that \href{https://etherscan.io/address/0xD7D08d621c125e0131689839639C52E714038b1f}{\texttt{0xD7D...b1f}} withdraws the same amount from TC during block $11{,}971{,}270$ and $11{,}972{,}098$, and then transfers $1{,}520$~\ETH to address \href{https://etherscan.io/address/0x36164B276EA6F7B1C00d8E27d4E7dC8f28035ac7}{\texttt{0x361...ac7}}, which finally exchanges all \ETH to fiat currency (e.g., \USD) on Houbi, a centralized exchange paltform. Given the address's registration information on Huobi, we can link the user's identity in the real world.

  \begin{figure}[h]
    \centering
    \includegraphics[width=0.8\columnwidth]{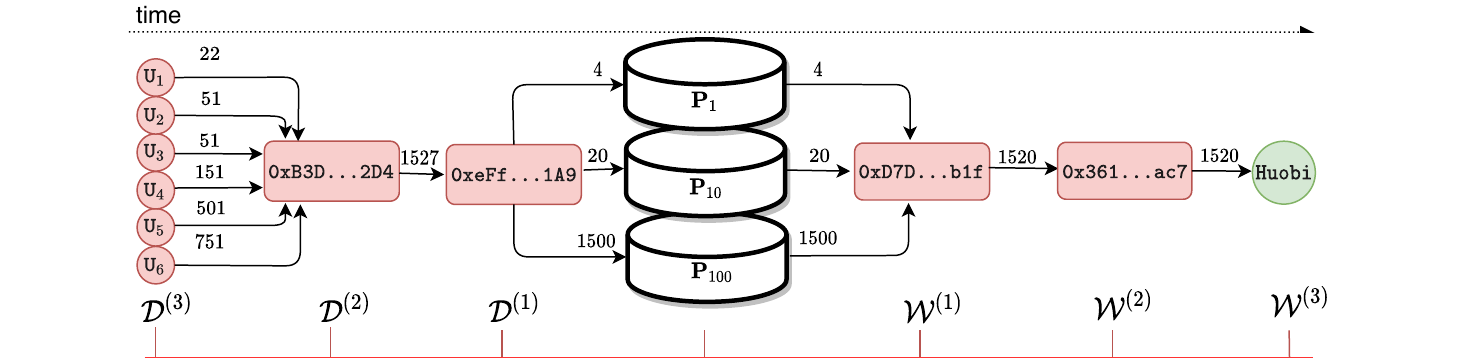}
    \caption{Example of tracing Upbit Hackers.}
    \label{fig:trace_upbit_hacker}
    \end{figure}
    \begin{figure}[h]
    \centering
    \includegraphics[width=0.8\columnwidth]{graph/tomato_hacker.pdf}
    \caption{Example of tracing Tomatos.Finance  Fishing addresses.}
    \label{fig:trace_tomato_hackers}
    \end{figure}

\pparagraph{Example 2: Tomatos.Finance Fishing} {\href{https://etherscan.io/address/0x917a417D938B9F9E6ae7F9e5253FB6DE410343e3}{0x917...3e3} is a labeled fishing address (\texttt{Fake\_Phishing4346}) which was used to steal users' funds on Tomatos.Finance.} We observe that this address leverages TC to launder money. As shown in Figure~\ref{fig:trace_tomato_hackers}, \emph{(1)} \href{https://etherscan.io/address/0x917a417D938B9F9E6ae7F9e5253FB6DE410343e3}{\texttt{Fake\_Phishing4346}} deposits $801.1~\ETH$ into TC 0.1, 1, and 100~\ETH pools during block $10{,}944{,}566$ and $10{,}944{,}735$. \emph{(2)} Through Heuristic~4, we find that the address \href{https://etherscan.io/address/0xB3D8Dc6b0C9fEc01aFBc69E282Ef720E2EF412D4}{\texttt{0xB3D...2D4}} withdraws the same amount of \ETH from the three TC pools after block $10{,}944{,}735$. Then \href{https://etherscan.io/address/0xB3D8Dc6b0C9fEc01aFBc69E282Ef720E2EF412D4}{\texttt{0xB3D...2D4}} is likely linked with \href{https://etherscan.io/address/0x917a417D938B9F9E6ae7F9e5253FB6DE410343e3}{\texttt{Fake\_Phishing4346}}. \emph{(3)} By manually checking the transactions of \href{https://etherscan.io/address/0xB3D8Dc6b0C9fEc01aFBc69E282Ef720E2EF412D4}{\texttt{0xB3D...2D4}}, we find that this address transfers $800~\ETH$ to \href{https://etherscan.io/address/0x00000000219ab540356cbb839cbe05303d7705fa}{\texttt{Eth2 Deposit Contract}} via $25$ transactions, and $0.97$~\ETH to \href{https://etherscan.io/address/0x6429C18067EE0bee037cE7A5DB7706e165E42Db1}{\texttt{0x642...Db1}}, which finally transfers funds to Coinbase, a centralized exchange platform. We can continue to trace the address given its information on Coinbase.
